# Supplementary material for: Multiple charge density waves and superconductivity nucleation at antiphase domain walls in the nematic pnictide Ba$_{1-x}$Sr$_{x}$Ni$_{2}$As$_{2}$
Source: arXiv:2102.03592 source file (2021-02-14)
Supplement: Supplementary file 1 [file Ba1-xSrxNi2As2_SI_v4.pdf]

# Supplementary Information: Three distinct charge density waves in the nematic pnictide superconductor $Ba_{1-x}Sr_xNi_2As_2$

## I. EXPERIMENTAL DETAILS

Single crystals of $Ba_{1-x}Sr_xNi_2As_2$ with $x = 0$, $0.27 \pm 0.01$, $0.42 \pm 0.01$, $0.47 \pm 0.01$, $0.65 \pm 0.02$, and $0.73 \pm 0.02$ were synthesized using the self-flux method reported in Ref. [1]. The precise chemical compositions were determined by energy dispersive x-ray spectroscopy on multiple spots on each sample. Single crystal x-ray scattering measurements were carried out using the in-lab x-ray instrument equipped with a Xenocs GeniX3D Mo $K_\alpha$ microspot x-ray source with multilayer focusing optics, providing $2.5 \times 10^7$ photons/sec in a beam spot of 130 $\mu$m at the sample position. The samples were cooled by a closed-cycle helium cryostat with a base temperature of 8 K mounted to a Huber four-circle diffractometer. The momentum resolution varied between $\Delta q = 0.01$ Å$^{-1}$ and 0.08 Å$^{-1}$ depending on the location in momentum space. Scattering signals were collected by a Mar345 image plate detector with 3450×3450 pixels. Three-dimensional surveys of momentum space were performed by taking images in 0.05° increments while sweeping samples through an angular range of 20° and mapping each pixel to the corresponding location in momentum space.

## II. LATTICE PARAMETERS

Lattice parameters of $Ba_{1-x}Sr_xNi_2As_2$ samples in high-temperature tetragonal phase and low-temperature triclinic phase are determined using single crystal x-ray diffraction measurements with Mo $K_\alpha$ x-ray source (Table S1). The crystal structure of the low-temperature phase of $BaNi_2As_2$ is reported to be triclinic structure with $P\bar{1}$ symmetry by by a previous structural refinement study in Ref. [2]. In this study, we used the standardized unit cell of the triclinic structure reported in Ref. [2]. Comparisons between the unit cell reported in Ref. [2] and the standardized unit cell can be found in the supplemental material of Ref. [3].

TABLE S1. Lattice parameters of $Ba_{1-x}Sr_xNi_2As_2$. Tetragonal lattice parameters are measured at room temperature and triclinic parameters at 50 K (except for $x = 0.42$, which is measured at 70 K).

| | Tetragonal structure | | Triclinic structure | | | | | |
|---|---|---|---|---|---|---|---|---|
| $x$ | a (Å) | c (Å) | a (Å) | b (Å) | c (Å) | $\alpha$ (°) | $\beta$ (°) | $\gamma$ (°) |
| 0 | 4.142(4) | 11.650(3) | 4.21(3) | 3.99(2) | 6.31(1) | 105.2(3) | 108.6(2) | 89.3(4) |
| 0.27 | 4.145(3) | 11.499(3) | 4.158(5) | 4.155(6) | 6.388(8) | 108.2(1) | 109.8(1) | 89.2(2) |
| 0.42 | 4.138(5) | 11.271(3) | 4.157(3) | 4.13(1) | 6.272(7) | 108.5(2) | 109.4(1) | 89.7(1) |
| 0.47 | 4.137(7) | 11.211(5) | 4.146(8) | 4.10(2) | 6.313(4) | 109.12(7) | 110.6(1) | 89.2(2) |
| 0.65 | 4.140(1) | 10.928(3) | 4.126(8) | 4.06(3) | 6.16(1) | 109.6(2) | 109.5(1) | 89.8(1) |
| 0.73 | 4.150(4) | 10.812(5) | - | - | - | - | - | - |

## III. STRUCTURAL PHASE TRANSITION IN $Ba_{0.58}Sr_{0.42}Ni_2As_2$

The tetragonal-to-triclinic structural phase transition in $Ba_{0.58}Sr_{0.42}Ni_2As_2$ is summarized in Fig. S1. When cooled across the phase transition, the $(0, 1, 9)_{\rm tet}$ structural Bragg reflection in the tetragonal phase splits into four reflections due to the formation of twin domains in triclinic phase [Fig. S1(a)]. One domain is chosen among the four, and the reflection of the domain is indexed as $(-1, 0, 5)_{\rm tri}$. The line scans through $(0, 1, 9)_{\rm tet}$ and $(-1, 0, 5)_{\rm tri}$ show a sharp transition in their integrated intensity at $T_s = 112.5 \pm 2.5$ K, indicating the change in symmetry of crystal structure [Figs. S1(b), (c)].

## IV. SYMMETRY PATTERN OF IC-CDW

The IC-CDW exhibits a peculiar symmetry pattern that, in a given Brillouin zone (BZ), the satellite reflections appear only one direction, either along $H$ or $K$ direction. However the direction is not unique: the satellites appear

at $(\pm 0.28, 0, 0)_{\rm tet}$ in some BZs, and at $(0, \pm 0.28, 0)_{\rm tet}$ in others. Fig. S2 shows the directionality of the IC-CDW in $H$-$K$ maps at odd-numbered $L$ in several different BZs measured in $Ba_{1-x}Sr_xNi_2As_2$, $x$ = 0, 0.27, 0.42, 0.47. By combining the patterns shown in Fig. S2 together, and assuming that the BZ at $\boldsymbol{Q}$ has the same pattern as the BZ at $-\boldsymbol{Q}$, we obtained the symmetry pattern of the IC-CDW in $H$-$K$ plane at odd-numbered $L$ (Fig. 3 in the main text). Due to not enough data, we could not determine the symmetry pattern at even-numbered $L$.

## V. UNIDIRECTIONALITY OF C-CDW-1 AND C-CDW-2

The satellite reflections of C-CDW-1 and C-CDW-2 appear in $K$ direction, not in $H$ direction, indicating that they are unidirectional. Fig. S3(a) shows the C-CDW-1 reflections in multiple Brillouin zones (BZs) at $(0, \pm 1/3, 0)_{\rm tri}$ and none is observed at $(\pm 1/3, 0, 0)_{\rm tri}$. Similarly, the C-CDW-2 reflections are observed at $(0, \pm 1/2, 0)_{\rm tri}$, not at $(\pm 1/2, 0, 0)_{\rm tri}$, in multiple BZs [Fig. S3(b)]. Thus, we conclude that the C-CDW-1 and C-CDW-2 are unidirectional, which is consistent with the fact that the underlying lattice is in triclinic phase, in which $C4$ symmetry is broken.

## VI. THEORY OF SUPERCONDUCTIVITY ON PERIOD-2 CDW DOMAIN WALLS

In this section we present details of the Landau-Ginzburg theory of superconductivity induced on domain walls of a period-2 CDW. Since the experimentally observed period-2 CDW is manifestly unidirectional we will present a simple one-dimensional theory. This can be easily extended to more complex orders with several CDW ordering wave vectors.

Following the work of McMillan [4], we represent the CDW as a modulation of the local charge density $\rho(x)$ of the form

$$\rho(x) = \rho_0 + \psi(x) e^{iQx} + \psi^*(x) e^{-iQx} + \text{higher harmonics} \tag{1}$$

where $\rho_0$ is the average charge density and $\psi(x)$ is the (generally complex) CDW order parameter. However in the period-2 case $Q = \pi$ (in units in which the lattice constant is set to unity), i.e. is a vector at the boundary of the Brillouin Zone. Hence, in this case the CDW order parameter is *real*, $\psi(x) = \psi^*(x)$, and it is slowly varying at the scale of the lattice spacing. We will also assume that there is a competing (also inhomogeneous) superconducting state represented by a local SC complex order parameter (the pairing amplitude) $\Delta(x)$ which, as we will see is not generally constant. We will be interested in the case in which the period-2 CDW is the "stronger order" and that it turns on at a higher temperature than the weaker SC order, $T_c^{\rm CDW} > T_c^{\rm SC}$. We will make use of gauge invariance of the SC order to work in the London gauge in which the SC order parameter is also real, $\Delta = \Delta^*$.

These assumptions lead us to the simplest possible form of the Landau-Ginzburg theory with competing CDW and SC orders whose free energy has the form

$$F = \int dx \left\{ \frac{K_{\rm CDW}}{2} (\partial_x \psi(x))^2 + \frac{r_{\rm CDW}}{2} \psi^2(x) + \frac{u_{\rm CDW}}{4} \psi^4(x) + \frac{K_{\rm SC}}{2} (\partial_x \Delta(x))^2 + \frac{r_{\rm SC}}{2} \Delta^2(x) + \frac{u_{\rm SC}}{4} \Delta^4(x) + \gamma\, \psi^2(x) \Delta^2(x) \right\} \tag{2}$$

Here $K_{\rm CDW}$ and $K_{\rm SC}$ are the stiffnesses of the CDW and the SC order parameters, respectively, and

$$r_{\rm CDW} = a_{\rm CDW}(T - T_c^{\rm CDW}), \qquad r_{\rm SC} = a_{\rm SC}(T - T_c^{\rm SC}) \tag{3}$$

We will assume that the coupling constants $u_{\rm CDW} > 0$ and $u_{\rm SC} > 0$, but we will allow the biquadratic coupling constant $\gamma$ to have either sign (provided its magnitude is not too large). We will be interested in the regime in which the system is in the period-2 CDW phase but above the uniform SC state. Thus, $T_c^{\rm SC} < T < T_c^{\rm CDW}$, and in this regime $r_{\rm CDW} < 0$ and $r_{\rm SC} > 0$.

The free energy of Eq.(2) is in the simplest form that one can write, but one could also consider additional terms. For instance, in Ref.[5] Chen and coworkers considered a biquadratic term with two derivatives of the form $\mu\, \Delta^2(x)\, (\partial_x \psi(x))^2$. For $\mu < 0$ (and large enough) such a term can favor the spontaneous formation of CDW domain walls with local SC order. On the other hand, unless one thinks that this term is due to disorder (see below), the resulting CDW state will be weakly incommensurate, which is not what is seen (thus far) in the low temperature regime of the period-2 state of $Ba_{1-x}Sr_xNi_2As_2$. In addition, while it is true that these gradient terms can lea to inhomogeneous states, it is difficult in practice to reach a regime in which $|\mu|$ is large enough (in virtue of the gradient coupling form of this term). We should note that if the CDW order has a period other than 2, its order parameter is complex and, in this case, the natural topological defects of the CDW are *discommensurations* at which the *phase* of its order parameter changes by $2\pi$, while the amplitude remains unchanged [6]. Thus, in the case of a commensurate

CDW with a wave vector not at the boundary of the Brillouin Zone the scheme that we consider here is not operative but it can be achieved again if one considers a large enough gradient coupling. Finally, we are also not including other interesting physical effects such as the presence of a metallic component which can lead to interesting temperature dependences of the ordering wave vector, among other things.

Here we will assume that the domain walls are due to the presence of disorder. Indeed, impurities generate local random potentials $V_{\rm dis}(x)$ which couple linearly to the local charge density $\rho(x)$ and hence also couple linearly to the CDW order parameter. Since in the period-2 case the order parameter is real, this coupling is analogous to the problem of an uniaxial ferromagnet (and Ising model) coupled to a local random field. A general argument by Imry and Ma [7] shows that a random field destroys long-range order in the 2D Ising model (and in any dimension below 4 for the incommensurate case) driven by the proliferation of domain walls. In three dimensions, in the commensurate case the domain walls proliferate only if the disorder is strong enough and there is a phase transition between the ordered and the disordered state (for a review see Ref. [8]). On the other hand, in a layered system the 2D to 3D crossover leads to a broad fluctuational regime. Pnictides are anisotropic but not layered so they are regarded as an intermediate case in which nevertheless these fluctuations are significant particularly in doped systems. The upshot of this analysis is that in the period-2 CDW phase of $\mathrm{Ba}_{1-x}\mathrm{Sr}_x\mathrm{Ni}_2\mathrm{As}_2$ one expects a significant number of antiphase domain walls.

We will now show that domain walls of $\mathrm{Ba}_{1-x}\mathrm{Sr}_x\mathrm{Ni}_2\mathrm{As}_2$ are actually superconducting. For simplicity we will consider a unidirectional period-2 CDW with a single domain wall. To this effect let us consider the Landau-Ginzburg equations for the free energy of Eq.(2). They are

$$-K_{\rm CDW}\partial_x^2\psi(x)+r_{\rm CDW}\psi(x)+u_{\rm CDW}\psi^3(x)+\gamma\psi(x)\Delta^2(x)=0, \tag{4}$$

$$-K_{\rm SC}\partial_x^2\Delta(x)+r_{\rm SC}\Delta(x)+u_{\rm SC}\Delta^3(x)+\gamma\psi^2(x)\Delta(x)=0 \tag{5}$$

In the regime $r_{\rm CDW}<0$ we will look for solutions with $\psi\neq 0$ and $\Delta(x)\neq 0$ satisfying the boundary conditions

$$\lim_{x\to\pm\infty}\psi(x)=\pm\psi_0, \qquad \lim_{x\to\pm\infty}\Delta(x)=0 \tag{6}$$

where $\psi_0=\sqrt{|r_{\rm CDW}|/u_{\rm CDW}}$ is the value of the period-2 CDW order parameter in the absence of the wall; in this regime, $r_{\rm SC}>0$, there is no uniform superconductivity and $\Delta=\Delta_0=0$.

We will consider the simpler case in which the stiffnesses of the CDW and the SC order parameters are the same, i.e. $K_{\rm CDW}=K_{\rm SC}\equiv K$. Furthermore, we will also require the quartic and biquadratic coupling constants to satisfy $u_{\rm CDW}=u_{\rm SC}=2\gamma\equiv u$, by which these couplings become $\frac{u}{4}(\psi^2+\Delta^2)^2$. With these assumptions the free energy of Eq.(2) simplifies,

$$F=\int dx\,\Big[\frac{K}{2}[(\partial_x\psi)^2+(\partial_x\Delta)^2]+\frac{1}{2}(r_{\rm CDW}\psi^2+r_{\rm SC}\Delta^2)+\frac{u}{4}(\psi^2+\Delta^2)^2\Big] \tag{7}$$

Next, we define the two-component real field

$$\boldsymbol{n}(x)=(\psi(x),\Delta(x))=\psi_0(\cos\theta,\sin\theta) \tag{8}$$

where we used the fact that in the regime of interest the CDW order is dominant. Here we will be interested in the case in which $0\leq\theta\leq\pi$, which means that $\psi$ takes values between $\pm\psi_0$. The free energy now becomes

$$F=\int dx\Big[\frac{\kappa}{2}(\partial_x\theta)^2-h\cos 2\theta+\varepsilon_0\Big] \tag{9}$$

where we used the following expressions for the effective stiffness $\kappa$, the anisotropy coupling constant $h$, and the uniform free energy density $\varepsilon_0$

$$\kappa\equiv K\psi_0^2=-\frac{K}{2u}(r_{\rm CDW}+r_{\rm SC})>0, \qquad h\equiv\frac{1}{8u}(r_{\rm CDW}^2-r_{\rm SC}^2)>0, \qquad \varepsilon_0\equiv-\frac{(r_{\rm CDW}+r_{\rm SC}))^2}{4u} \tag{10}$$

where we used that $r_{\rm CDW}<0$ and $|r_{\rm CDW}|>r_{\rm SC}>0$, and that in the uniform equilibrium broken symmetry state

$$\psi_0^2=-\frac{(r_{\rm CDW}+r_{\rm SC})}{u}>0 \tag{11}$$

The Landau-Ginzburg equation for the simplified free energy of Eq.(9) is

$$-\kappa\partial_x^2\theta+2h\sin 2\theta=0 \tag{12}$$

which, for $h > 0$ (dominant CDW) has the uniform solutions $\theta = 0, \pi$ corresponding to $\psi = \pm\psi_0$, respectively (and no superconductivity).

There is, however, a non-trivial domain wall solution of Eq.(12) which interpolates between these two uniform states. To find the solution we use the standard analogy by which we will regard the coordinate $x$ as "time". In this picture Eq.(12) is regarded as the equation of motion of a "physical pendulum" whose degree of freedom is the angle $\theta$. The "energy" of the pendulum is

$$E = \frac{\kappa}{2}(\partial_x \theta)^2 + h\cos 2\theta \tag{13}$$

The energy of the pendulum for the uniform solutions $\theta = 0, \pi$ is just $h$. There is another solution also with energy $h$ which satisfies

$$\frac{\kappa}{2}(\partial_x \theta)^2 + h\cos 2\theta = h \tag{14}$$

or, what is the same as

$$(\partial_x \theta)^2 = 2\frac{h}{\kappa}(1 - \cos 2\theta) \tag{15}$$

This is equivalent to the first order differential equations

$$\partial_x \theta = \pm 2\sqrt{\frac{h}{\kappa}}\sin\theta \tag{16}$$

The solutions to this first order differential equation are

$$\theta_\pm(x) = 2\tan^{-1}\left(e^{\pm 4\sqrt{\frac{h}{\kappa}}x}\right) \tag{17}$$

where we set the arbitrary origin at $x = 0$, where $\theta_\pm(0) = \frac{\pi}{2}$. After some algebra we find that the domain wall solutions for the CDW and SC order parameters are

$$\psi(x) = \pm\psi_0 \tanh\left(4\sqrt{\frac{h}{\kappa}}x\right), \qquad \Delta(x) = \frac{\psi_0}{\cosh\left(4\sqrt{\frac{h}{\kappa}}x\right)} \tag{18}$$

Clearly, the solution with positive sign interpolates between $\theta = \pi$, i.e. $\psi \to \psi_0$ as $x \to -\infty$, and $\theta = 0$, i.e. $\psi \to +\psi_0$ as $x \to +\infty$. This solution describes the domain wall (the solution with the negative sign describes the anti-domain wall). It is apparent that far from the domain wall the CDW order parameter becomes $\pm\psi_0$ and approaches these values exponentially fast. Conversely, the SC order parameter $\Delta$ vanishes exponentially fast far from the domain wall and reaches its maximum value, $\psi_0$ within our simplifications, at the location of the topological defect. The free energy cost of the domain wall per unit length (or area) of the wall is the difference of the free energy of Eq.(9) for these solutions relative to the uniform state and is given by $F_{\text{wall}} = 2\sqrt{h\kappa} > 0$.

In this derivation we assumed that $\gamma = 2u$ which means that the biquadratic term is as important as the usual quartic terms. However solutions of this type can be obtained in the more general case in which $\gamma$ is weak. In that case one can first find a CDW domain wall solution and then solve for the SC state nucleated at the wall (assuming that the back reaction is parametrically small). Since $T^c_{\text{CDW}} \gg T^c_{\text{SC}}$, we can find an approximate domain wall solution of Eqs.(4) and (5) that satisfy the domain wall boundary conditions, Eq.(6), by assuming that the coupling constant $\gamma$ in Eq.(4) is weak and then solve Eq.(5) in the background of the CDW domain wall. With this approximation, the solution to Eq.(4) that obeys the boundary condition of Eq.(6) is (centered arbitrarily at $x = 0$)

$$\psi(x) = \psi_0 \tanh(x/\xi_{\text{CDW}}) \tag{19}$$

where $\xi_{\text{CDW}} = |2K_{\text{CDW}}/r_{\text{CDW}}|^{1/2} \propto (T_c^{\text{CDW}} - T)^{-1/2}$ is the CDW correlation length and $\psi_0 = \sqrt{|r_{\text{CDW}}|/u_{\text{CDW}}}$ is the expectation value in the uniform unperturbed CDW state.

Eq.(5) in the background of the CDW domain wall, which now becomes

$$-K_{\text{SC}}\partial_x^2\Delta(x) + r_{\text{SC}}\Delta(x) + \gamma\psi_0^2(x)\tanh^2(x/\xi_{\text{CDW}})\,\Delta(x) + u_{\text{SC}}\Delta^3(x) = 0 \tag{20}$$

We will seek a solution with $\Delta(x) \neq 0$ with lower free energy than the domain wall without SC order. The SC order parameter $\Delta(x)$ will be vanishingly small near the onset of the SC state. In this regime we can look for solutions of the *linearized* equation with an arbitrary amplitude

$$-K_{\text{SC}}\partial_x^2\Delta(x) + r_{\text{SC}}\Delta(x) + \gamma\psi_0^2(x)\tanh^2(x/\xi_{\text{CDW}})\,\Delta(x) = 0 \tag{21}$$

and then fix the value of the amplitude by demanding that the free energy is minimized (including the non-linear term). Upon defining a rescaled coordinate $v = x/\xi_{\rm CDW}$, we can bring the linearized equation to the form of a Schrödinger equation of the form

$$-\frac{1}{2}\partial_v^2 \Delta(u) + U(v)\Delta(v) = E\Delta(v) \tag{22}$$

where we defined

$$U(v) \equiv -\frac{\lambda(\lambda+1)}{2}\frac{1}{\cosh^2 v}, \tag{23}$$

$$E \equiv -\frac{r_{\rm SC}+\gamma\psi_0^2}{2K_{\rm SC}}\,\xi_{\rm CDW}^2 \tag{24}$$

where $\lambda(\lambda+1) = \gamma\psi_0^2/K_{\rm SC}$.

Eq.(22) is the Schrödinger equation for a stationary state with energy $E$ in the Pöschl-Teller potential (given in Eq.(23)) [9]. The solutions are the Legendre functions $P_\lambda^\mu(v)$ where $E = -\mu^2/2$. This equation has a bound state with $E = -1/2$ and the solution is

$$\Delta(x) = \frac{A}{\cosh(x/\xi_{\rm CDW})} \tag{25}$$

where $A$ is a constant to be determined. The important feature of this solution is that it vanishes (exponentially fast) as $v \to \pm\infty$.

Using the expression for the induced SC order parameter, Eq.(25), we find that the free energy of the SC state localized on the domain wall is

$$F_{\rm SC} = \frac{2K_{\rm SC}}{\xi_{\rm CDW}}\Big[-\frac{1}{2}+\frac{(r_{\rm SC}+\gamma\psi_0^2)}{2K_{\rm SC}}\Big]\,A^2 + \frac{1}{3}\xi_{\rm SC}u_{\rm SC}\,A^4 \tag{26}$$

The SC state localized on the domain wall becomes favorable if the quantity in brackets in Eq.(26) becomes negative, or, what is the same as $E = -1/2$. Upon minimizing Eq.(26) we find that the amplitude $A$ is given by

$$A^2 = -\frac{3K_{\rm SC}}{u_{\rm SC}\xi_{\rm CDW}}\Big[-\frac{1}{2}+\frac{(r_{\rm SC}+\gamma\psi_0^2)}{2K_{\rm SC}}\Big] > 0 \tag{27}$$

It is apparent that solutions that we found in the regime $\gamma \ll u$, Eqs. (19) and (25), have the same form as in the regime $\gamma = 2u$ discussed above, Eq.(18), albeit with somewhat different parameters. There is, however, an important difference in this regime. By inspection we see that there is a critical temperature for the SC solution on the wall to exist, given by the condition that the quantity in brackets in Eq.(27) vanishes. This temperature is much lower than the critical temperature of the period 2 CDW state.

On the other hand, since the free energy of the SC wall solution is not zero, these topological defects of the CDW state cannot be formed spontaneously in the period 2 CDW ordered phase. However, disorder can (and does) favor the creation of domain walls. We noted in the text that disorder coupes to the period 2 CDW in the same way as a random field in an Ising ferromagnet. A standard argument due to Imry and Ma [7] shows that in two dimensions *any* amount of random field disorder destroys the long range ordered state, the period 2 CDW in this case, while in higher dimensions a critical amount of disorder is needed. In layered systems there is an intermediate broad fluctuational regime signaling the 2D to 3D crossover. However, while $Ba_{0.58}Sr_{0.42}Ni_2As_2$ is anisotropic, the anisotropy is not large enough to regard this system (as well as all pnictides) as being layered (in contrast with the cuprate superconductors). We should note that while it is reasonable to expect that doping could drive $Ba_{0.58}Sr_{0.42}Ni_2As_2$ weakly incommensurate by creation of domain walls (as in the McMillan scenario [6], so far there is no experimental indication of any incommensuration in the low temperature regime of the period 2 CDW state.

Therefore we conclude that a SC state will be nucleated at the antiphase domain walls of the period 2 CDW. We can regard this phenomenon as the onset of local superconductivity. However the thermodynamic transition to a macroscopic superconducting state will only happen at a substantially lower temperature driven by the Josephson coupling between nearby domain walls (see, e.g. Ref. [10]). We should note that the arguments presented here bear a close analogy with the theory of halos of SC vortices of Ref.[11] for the existence of CDW (charge) order in the

vicinity of a SC vortex.


[1] C. Eckberg, D. J. Campbell, T. Metz, J. Collini, H. Hodovanets, T. Drye, P. Zavalij, M. H. Christensen, R. M. Fernandes, S. Lee, P. Abbamonte, J. W. Lynn, and J. Paglione, Sixfold enhancement of superconductivity in a tunable electronic nematic system, Nature Physics **16**, 346 (2020).

[2] A. S. Sefat, M. A. McGuire, R. Jin, B. C. Sales, D. Mandrus, F. Ronning, E. D. Bauer, and Y. Mozharivskyj, Structure and anisotropic properties of $Ba_{1-x}Sr_xNi_2As_2$ single crystals, Phys. Rev. B **79**, 094508 (2009).

[3] S. Lee, G. de la Peña, S. X.-L. Sun, M. Mitrano, Y. Fang, H. Jang, J.-S. Lee, C. Eckberg, D. Campbell, J. Collini, J. Paglione, F. M. F. de Groot, and P. Abbamonte, Unconventional Charge Density Wave Order in the Pnictide Superconductor $Ba_{1-x}Sr_xNi_2As_2$, Phys. Rev. Lett. **122**, 147601 (2019).

[4] W. L. McMillan, Landau theory of charge density waves in transition-metal dichalcogenides, Phys. Rev. B **12**, 1187 (1975).

[5] C. Chen, L. Su, A. H. Castro Neto, and V. M. Pereira, Discommensuration-driven superconductivity in the charge density wave phases of transition-metal dichalcogenides, Phys. Rev. B **99**, 121108 (2019).

[6] W. L. McMillan, Theory of discommensurations and the commensurate-incommensurate charge-density-wave phase transition, Phys. Rev. B **14**, 1496 (1976).

[7] Y. Imry and S.-K. Ma, Random-Field Instability of the Ordered State of Continuous Symmetry, Phys. Rev. Lett. **35**, 1399 (1975).

[8] T. Nattermann, Theory of the Random Field Ising Model, in *Spin Glasses and Random Fields*, edited by A. P. Young (World Scientific, Singapore, 1998) pp. 277–298, arXiv:cond-mat/9705295.

[9] L. D. Landau and E. M. Lifshitz, *Quantum Mechanics: Non-Relativistic Theory*, third, revised and enlarged ed., Course of Theoretical Physics, Vol. v.3 (Butterworth-Heinemann, Oxford, 1991).

[10] V. J. Emery, E. Fradkin, S. A. Kivelson, and T. C. Lubensky, Quantum Theory of the Smectic Metal State in Stripe Phases, Phys. Rev. Lett. **85**, 2160 (2000).

[11] S. A. Kivelson, D.-H. Lee, E. Fradkin, and V. Oganesyan, Competing order in the mixed state of high-temperature superconductors, Phys. Rev. B **66**, 144516 (2002).

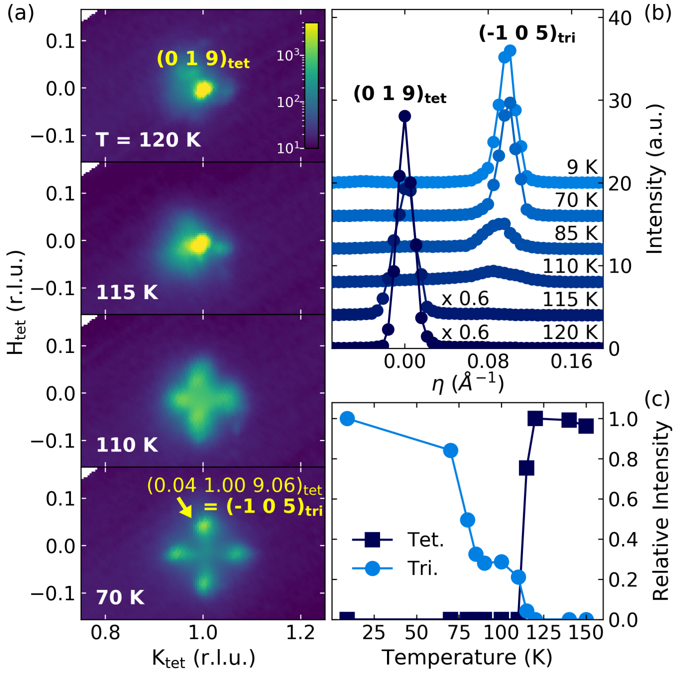


FIG. S1. Tetragonal-to-triclinic structural phase transition in $Ba_{0.58}Sr_{0.42}Ni_2As_2$. (a) $H$-$K$ maps at a selection of temperatures showing the evolution of $(0,1,9)_{\rm tet}$ structural Bragg reflection across the phase transition. The splitting of the reflection below $T = T_{\rm s}$ is due to the formation of twin domains in triclinic phase. (b) Line momentum scans through tetragonal $(0,1,9)_{\rm tet}$ and triclinic $(-1,0,5)_{\rm tri}$ Bragg reflections. $\eta$ is the distance in momentum space from $(0,1,9)_{\rm tet}$ along the direction to $(-1,0,5)_{\rm tri}$. (c) Integrated intensities of the tetragonal (Tet.) and triclinic (Tri.) Bragg reflections, showing the change in symmetry of crystal structure.

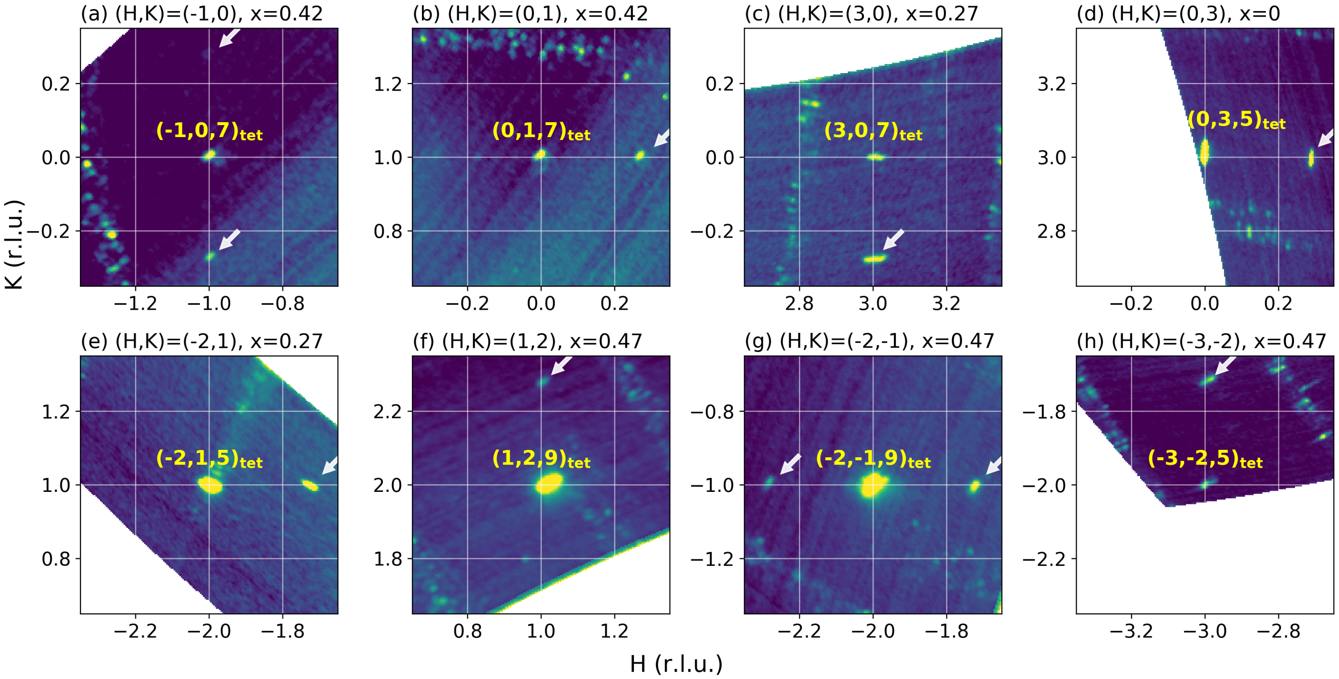


FIG. S2. Selected $H$-$K$ maps at odd-numbered $L$ of IC-CDW in several different Brillouin zones measured in $Ba_{1-x}Sr_xNi_2As_2$, $x = 0$, 0.27, 0.42, 0.47. The IC-CDW satellite reflections are indicated with white arrows. The indices of Brillouin zones and the Sr content $x$ are labeled in each panel.

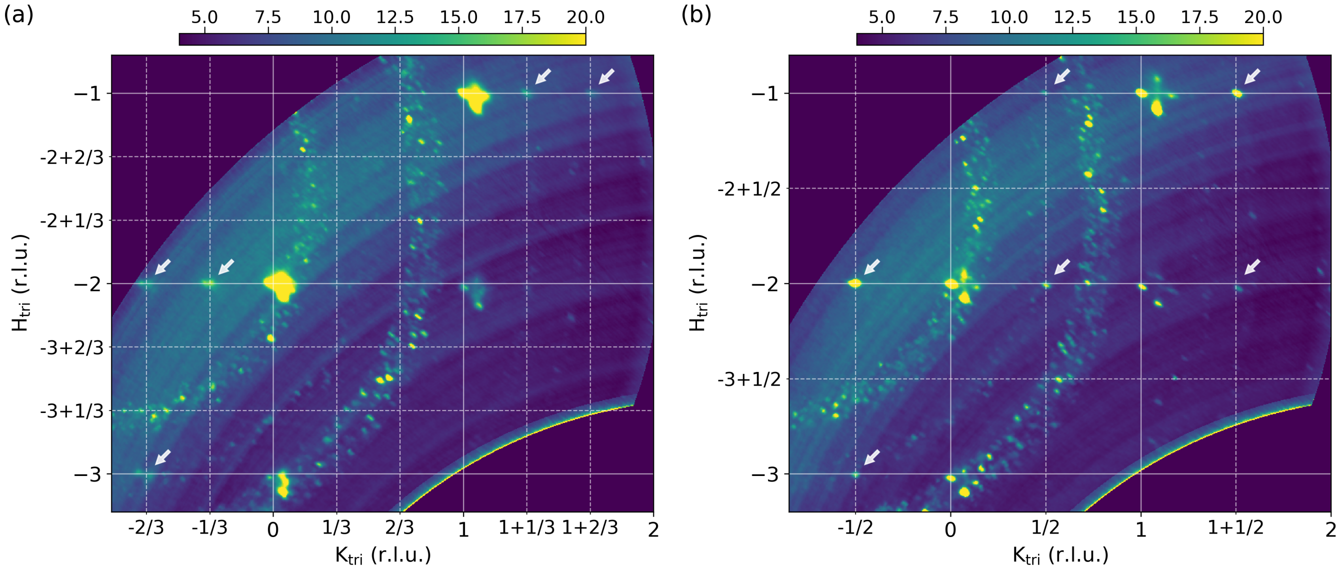


FIG. S3. (a) $H$-$K$ map at $L_{\mathrm{tri}} = 6$ of $Ba_{0.58}Sr_{0.42}Ni_2As_2$ at $T = 110$ K. C-CDW-1 satellite reflections appear at $(0, \pm1/3, 0)_{\mathrm{tri}}$ (white arrows), not at $(\pm1/3, 0, 0)_{\mathrm{tri}}$. (b) Similar map at $T = 9$ K, showing C-CDW-2 reflections at $(0, \pm1/2, 0)_{\mathrm{tri}}$ (white arrows), not at $(\pm1/2, 0, 0)_{\mathrm{tri}}$.
